# Supplementary material for: Design of platform trials with a change in the control treatment arm
Source: arXiv:2311.17467 source file (2023-11-29)
Supplement: Supplementary file 1 [file Supplementary_Materials___Design_of_platform_trials_with_a_change_in_the_control_treatment_arm.pdf]

# Supplementary Materials: Design of platform trials with a change in the control treatment arm

Peter Greenstreet<sup>1,2,\*</sup>, Thomas Jaki<sup>3,4</sup>, Alun Bedding<sup>5</sup>, Pavel Mozgunov<sup>3</sup>

<sup>1</sup> Department of Mathematics and Statistics, Lancaster University, Lancaster, UK

<sup>2</sup> Exeter CTU, University of Exeter, Exeter, UK

<sup>3</sup> MRC Biostatistics Unit, University of Cambridge, Cambridge, UK

<sup>4</sup> University of Regensburg, Regensburg, Germany

<sup>5</sup> Roche Products Ltd., Welwyn Garden City, UK

\* p.greenstreet@lancaster.ac.uk

## 1 Proof for conditional power Theorem 3.3

*Proof.* We define the following:

$$\begin{aligned} B_{k^*,j}(\delta_{1,j}, \delta_{2,j}) &= [-\infty < Z_{k^*,k',j}^* < (\delta_{2,j}u_j + \delta_{1,j})] \\ C_{k^*,j}(\delta_{1,j}, \delta_{2,j}) &= [(\delta_{2,j}u_j + \delta_{1,j}) < Z_{k^*,k',j}^*]. \end{aligned}$$

The conditional power equals is:

$$R(\delta_{1,j}, \delta_{2,j}) = \bigcup_{j=j'+1}^J \left[ \bigcap_{i=j'+1}^{j-1} (B_{k^*,i}(\delta_{1,i}, \delta_{2,i})) \cap C_{k^*,j}(\delta_{1,j}, \delta_{2,j}) \right]. \quad (1.1)$$

When no data is taken  $\delta_{1,j} = 0$  and  $\delta_{2,j} = 1$ . However when old data is taken forward  $\delta_{1,j} = \frac{-\hat{Z}_{k,k',j'}\sqrt{n_{k',j'}}}{\sqrt{n_{k,j}-n_{k,j'}}}$  and  $\delta_{2,j} = \frac{\sqrt{n_{k,j}}}{\sqrt{n_{k,j}-n_{k,j'}}}$ . Therefore when old data is retained  $\delta_{1,j} \geq 0$  and  $\delta_{2,j} \geq 1$  as  $\hat{Z}_{k,k',j'} < 0$ .

Then under the assumption  $u_j \geq 0$  for all  $j = (j' + 1) \dots J$ . For any  $\epsilon_{1,j} \geq 0$  and  $\epsilon_{2,j} \geq 0$  let

$$w = (Z_{k^*,k',j'+1}^*, \dots, Z_{k^*,k',J}^*) \in \bigcup_{j=j'+1}^J \left[ \bigcap_{i=j'+1}^{j-1} (B_{k^*,i}(\delta_{1,i} + \epsilon_{1,i}, \delta_{2,i} + \epsilon_{2,i})) \cap C_{k^*,j}(\delta_{1,j} + \epsilon_{1,j}, \delta_{2,j} + \epsilon_{2,j}) \right].$$

For some  $q \in \{j' + 1, \dots, J\}$  for which  $Z_{k^*,k',q}^* \in C_{k^*,q}(\delta_{1,q} + \epsilon_{1,q}, \delta_{2,q} + \epsilon_{2,q})$  and  $Z_{k^*,k',h}^* \in B_{k^*,h}(\delta_{1,h} + \epsilon_{1,h}, \delta_{2,h} + \epsilon_{2,h})$  for  $h = j' + 1, \dots, q - 1$ .  $Z_{k^*,k',q}^* \in C_{k^*,q}(\delta_{1,q} + \epsilon_{1,q}, \delta_{2,q} + \epsilon_{2,q})$  implies that  $Z_{k^*,k',q}^* \in C_{k^*,q}(\delta_{1,q}, \delta_{2,q})$ . Furthermore  $Z_{k^*,k',q}^* \in B_{k^*,q}(\delta_{1,q} + \epsilon_{1,q}, \delta_{2,q} + \epsilon_{2,q})$  implies that  $Z_{k^*,k',q}^* \in B_{k^*,q}(\delta_{1,q}, \delta_{2,q}) \cup C_{k^*,q}(\delta_{1,q}, \delta_{2,q})$  for some  $h = j' + 1, \dots, q - 1$ . Therefore,

$$w = (Z_{k^*,k',j'+1}^*, \dots, Z_{k^*,k',J}^*) \in \bigcup_{j=j'+1}^J \left[ \bigcap_{i=j'+1}^{j-1} (B_{k^*,i}(\delta_{1,i}, \delta_{2,i})) \cap C_{k^*,j}(\delta_{1,j}, \delta_{2,j}) \right]. \quad (1.2)$$

As a result  $P(R(0,1)) \geq P(R(\frac{-\hat{Z}_{k,k',j'}\sqrt{n_{k',j'}}}{\sqrt{n_{k,j}-n_{k,j'}}}, \frac{\sqrt{n_{k,j}}}{\sqrt{n_{k,j}-n_{k,j'}}}))$ .  $\square$

## 2 Conditional power formulations for Case 1

The denominator of the conditional power for a change after the first stage is:

$$P(E_{k^*,k',1}^1 \cap E_{k^*,k',1}^2 \cap E_{k^*,k',1}^3) = \int_{u_1}^{\infty} \int_{l_1}^{\infty} \int_{-\infty}^0 \int_{-\infty}^0 \phi \left[ \mathbf{z}, \mu_{[1,2,3,4]}^{\Omega_{k^*,k',1}}, \Sigma_{[1,2,3,4]}^{\Omega_{k^*,k',1}} \right] \mathbf{dz}. \quad (2.1)$$

where  $\phi(\mathbf{z}, \mu, \Sigma)$  is the probability density function of a multi-variate normal distribution with mean  $\mu$  and covariance matrix  $\Sigma$ . Also

$$\mu^{\Omega_{k^*,k',1}} = \left( \frac{\sqrt{n}(\mu_{k'} - \mu_0)}{\sigma\sqrt{2}}, \frac{\sqrt{n}(\mu_{k^*} - \mu_0)}{\sigma\sqrt{2}}, \frac{\sqrt{n}(\mu_{k^*} - \mu_{k'})}{\sigma\sqrt{2}}, \frac{\sqrt{n}(\mu_k - \mu_{k'})}{\sigma\sqrt{2}}, \frac{\sqrt{n}(\mu_{k^*} - \mu_{k'})}{\sigma} \right),$$

and

$$\Sigma^{\Omega_{k^*,k',1}} = \begin{pmatrix} 1 & \frac{1}{2} & -\frac{1}{2} & -\frac{1}{2} & -\frac{1}{2}\sqrt{\frac{1}{2}} \\ \frac{1}{2} & 1 & \frac{1}{2} & 0 & \frac{1}{2}\sqrt{\frac{1}{2}} \\ -\frac{1}{2} & \frac{1}{2} & 1 & \frac{1}{2} & \sqrt{\frac{1}{2}} \\ -\frac{1}{2} & 0 & \frac{1}{2} & 1 & \frac{1}{2}\sqrt{\frac{1}{2}} \\ -\frac{1}{2}\sqrt{\frac{1}{2}} & \frac{1}{2}\sqrt{\frac{1}{2}} & \sqrt{\frac{1}{2}} & \frac{1}{2}\sqrt{\frac{1}{2}} & 1 \end{pmatrix},$$

with  $[\cdot]$  defining which entries to take from the vector, and  $[\cdot]$  also defines the rows and columns of the matrix, needed. The numerator of the conditional power for a change after the first stage is:

$$P(E_{k^*,k',1}^1 \cap E_{k^*,k',1}^2 \cap E_{k^*,k',1}^3 \cap E_{k^*,k',1}^4) = \int_{u_1}^{\infty} \int_{l_1}^{\infty} \int_{-\infty}^0 \int_{-\infty}^0 \int_{u_2}^{\infty} \phi \left[ \mathbf{z}, \mu^{\Omega_{k^*,k',1}}, \Sigma^{\Omega_{k^*,k',1}} \right] \mathbf{dz}. \quad (2.2)$$

The conditional power for treatment  $k^*$  when treatment  $k'$  becomes the new control at stage 1 equals Equation (2.2) divided by Equation (2.1). When only retaining the new information the conditional power is:

$$P(E_{k^*,k',1}^{*4}) = \int_{u_2}^{\infty} \phi \left[ \mathbf{z}, \left( \frac{\sqrt{n}(\mu_{k^*} - \mu_{k'})}{\sigma\sqrt{2}} \right), 1 \right] \mathbf{dz}. \quad (2.3)$$

## 3 Overall power formulations for Case 1

Due to all the arms starting at the same point  $\Xi_{k,1}$  can be simplified to

$$\Xi_{k,1} = \int_{u_1}^{\infty} \int_{-\infty}^0 \int_{-\infty}^0 \phi \left[ \mathbf{z}, \mu^{\Xi_{k,1}}, \Sigma^{\Xi_{k,1}} \right] \mathbf{dz},$$

where

$$\mu^{\Xi_{k,1}} = \left( \frac{\sqrt{n}(\mu_{k^*} - \mu_0)}{\sigma\sqrt{2}}, \frac{\sqrt{n}(\mu_{k_1} - \mu_{k^*})}{\sigma\sqrt{2}}, \frac{\sqrt{n}(\mu_{k_2} - \mu_{k^*})}{\sigma\sqrt{2}} \right),$$

and

$$\Sigma^{\Xi_{k,1}} = \begin{pmatrix} 1 & -\frac{1}{2} & -\frac{1}{2} \\ -\frac{1}{2} & 1 & \frac{1}{2} \\ -\frac{1}{2} & \frac{1}{2} & 1 \end{pmatrix}.$$

The probability  $k^*$  becomes the control at the second stage is

$$\begin{aligned} \Xi_{k,2} = & \int_{l_1}^{u_1} \int_{u_2}^{\infty} \int_{-\infty}^{l_1} \int_{-\infty}^{l_1} \phi \left[ \mathbf{z}, \mu_{[1,2,3,5]}^{\Xi_{k,2}}, \Sigma_{[1,2,3,5]}^{\Xi_{k,2}} \right] \mathbf{dz} + \int_{l_1}^{u_1} \int_{u_2}^{\infty} \int_{l_1}^{u_1} \int_{-\infty}^0 \int_{-\infty}^{l_1} \phi \left[ \mathbf{z}, \mu_{[1,2,3,4,5]}^{\Xi_{k,2}}, \right. \\ & \Sigma_{[1,2,3,4,5]}^{\Xi_{k,2}} \left. \right] \mathbf{dz} + \int_{l_1}^{u_1} \int_{u_2}^{\infty} \int_{-\infty}^{l_1} \int_{l_1}^{u_1} \int_{-\infty}^0 \phi \left[ \mathbf{z}, \mu_{[1,2,3,5,6]}^{\Xi_{k,2}}, \Sigma_{[1,2,3,5,6]}^{\Xi_{k,2}} \right] \mathbf{dz} \\ & + \int_{l_1}^{u_1} \int_{u_2}^{\infty} \int_{l_1}^{u_1} \int_{-\infty}^0 \int_{l_1}^{u_1} \int_{-\infty}^0 \phi \left[ \mathbf{z}, \mu^{\Xi_{k,2}}, \Sigma^{\Xi_{k,2}} \right] \mathbf{dz}, \end{aligned}$$

where

$$\mu^{\Xi_{k,2}} = \left( \frac{\sqrt{n}(\mu_{k^*} - \mu_0)}{\sigma\sqrt{2}}, \frac{\sqrt{n}(\mu_{k^*} - \mu_0)}{\sigma}, \frac{\sqrt{n}(\mu_{k_1} - \mu_0)}{\sigma\sqrt{2}}, \frac{\sqrt{n}(\mu_{k_1} - \mu_{k^*})}{\sigma}, \frac{\sqrt{n}(\mu_{k_2} - \mu_0)}{\sigma\sqrt{2}}, \frac{\sqrt{n}(\mu_{k_2} - \mu_{k^*})}{\sigma} \right),$$

and

$$\Sigma^{\Xi_{k,2}} = \begin{pmatrix} 1 & \sqrt{\frac{1}{2}} & \frac{1}{2} & -\frac{1}{2}\sqrt{\frac{1}{2}} & \frac{1}{2} & -\frac{1}{2}\sqrt{\frac{1}{2}} \\ \sqrt{\frac{1}{2}} & 1 & \frac{1}{2}\sqrt{\frac{1}{2}} & -\frac{1}{2} & \frac{1}{2}\sqrt{\frac{1}{2}} & -\frac{1}{2} \\ \frac{1}{2} & \frac{1}{2}\sqrt{\frac{1}{2}} & 1 & \frac{1}{2}\sqrt{\frac{1}{2}} & \frac{1}{2} & 0 \\ -\frac{1}{2}\sqrt{\frac{1}{2}} & -\frac{1}{2} & \frac{1}{2}\sqrt{\frac{1}{2}} & 1 & 0 & \frac{1}{2} \\ \frac{1}{2} & \frac{1}{2}\sqrt{\frac{1}{2}} & \frac{1}{2} & 0 & 1 & \frac{1}{2}\sqrt{\frac{1}{2}} \\ -\frac{1}{2}\sqrt{\frac{1}{2}} & -\frac{1}{2} & 0 & \frac{1}{2} & \frac{1}{2}\sqrt{\frac{1}{2}} & 1 \end{pmatrix}.$$

We have  $\Omega_{k^*,k',1}$  equals Equation (2.2) and  $\Omega_{k^*,k',1}^*$  equals Equation (2.1) multiplied by Equation (2.3).

## 4 The effect of different values of $\mu_3 - \mu_0$ for the Case 1

The results of using different values of  $\mu_3 - \mu_0$  are studied. The values studied are  $\mu_3 - \mu_0 = -\theta_0$ ,  $\mu_3 - \mu_0 = 0$  and  $\mu_3 - \mu_0 = \theta_0$ . The conditional power for treatment 2 given treatment 1 has become the new control at stage 1 when using all the data is given in Figure 1. The conditional power for treatment 2 given treatment 1 has become the new control at stage 1 when using only the new data is given in Figure 2. The difference in conditional power for treatment 2 given treatment 1 has become the new control at stage 1 is given in Figure 3. The overall power when using all the data is given in Figure 4. The overall power when using only the new data is given in Figure 5. The difference in overall power is given in Figure 6. The probability of the treatment which does not have the greatest treatment effect becoming the control at the first stage is given in Figure 7.

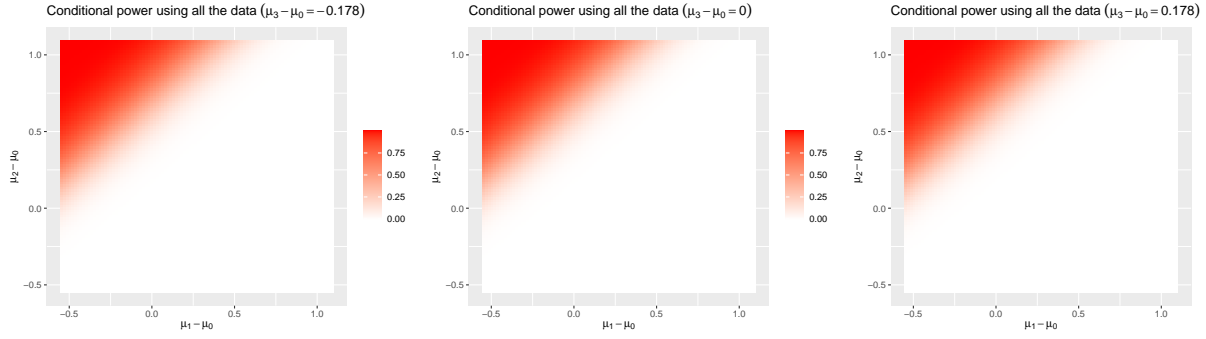

Figure 1: For multiple values of  $\mu_3 - \mu_0$ : the conditional power for treatment 2 given that treatment 1 has gone forward at the first stage when all the data is retained.

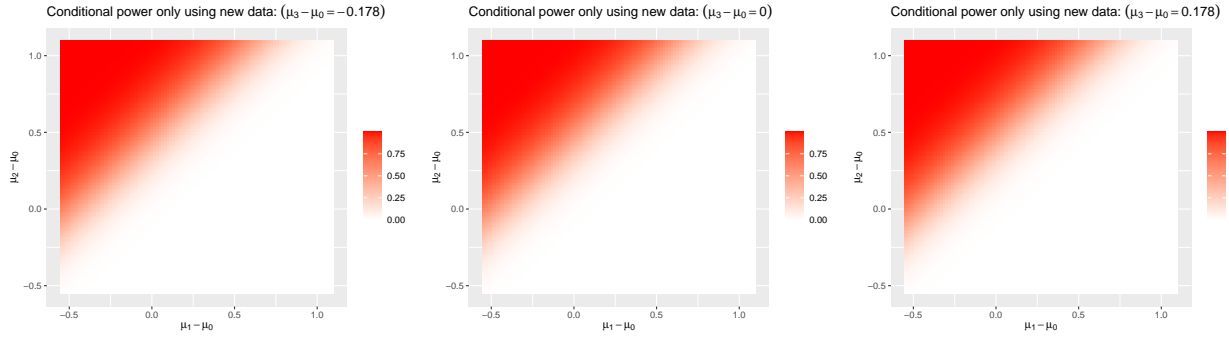

Figure 2: For multiple values of  $\mu_3 - \mu_0$ : the conditional power for treatment 2 given that treatment 1 has gone forward at the first stage when only the data post the change in control is used.

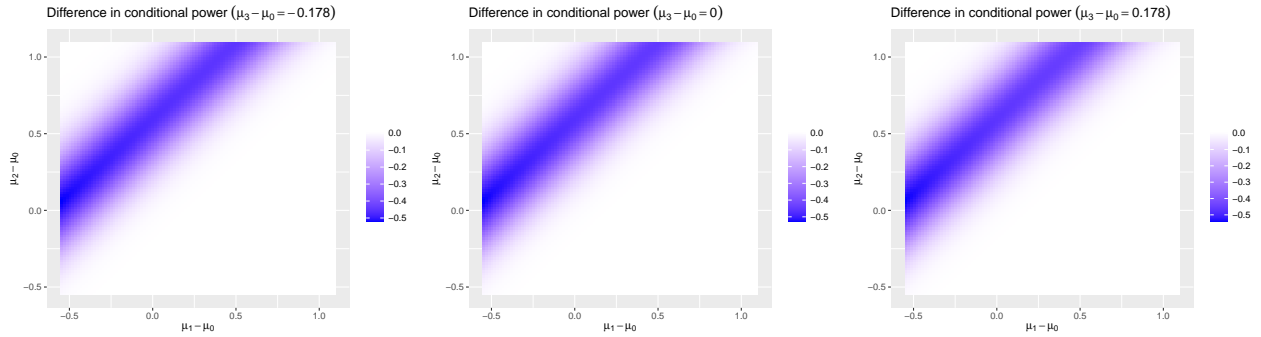

Figure 3: For multiple values of  $\mu_3 - \mu_0$ : the difference in conditional power between keeping the data pre change and not.

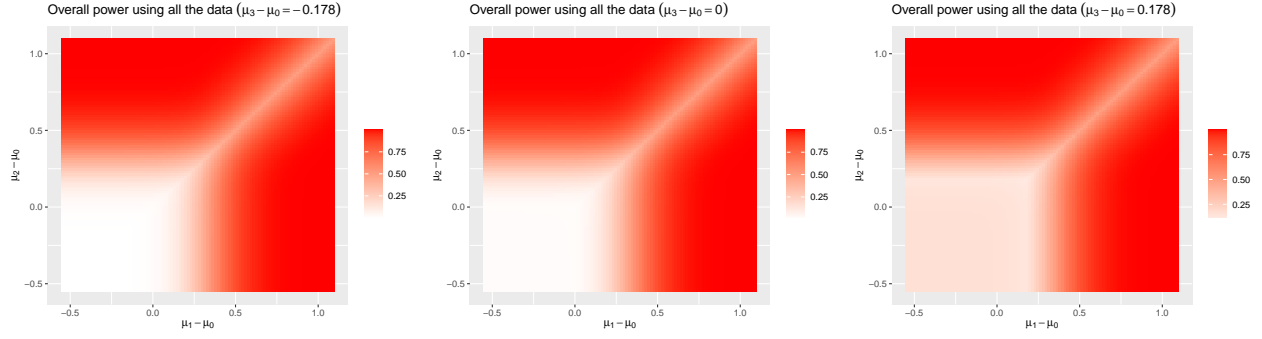

Figure 4: For multiple values of  $\mu_3 - \mu_0$ : the overall power when all the data is retained.

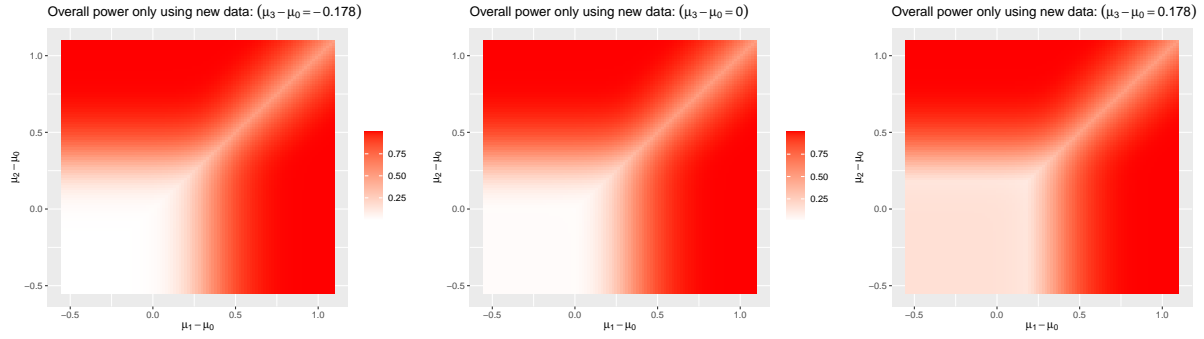

Figure 5: For multiple values of  $\mu_3 - \mu_0$ : the overall power when only the data post the change in control is used.

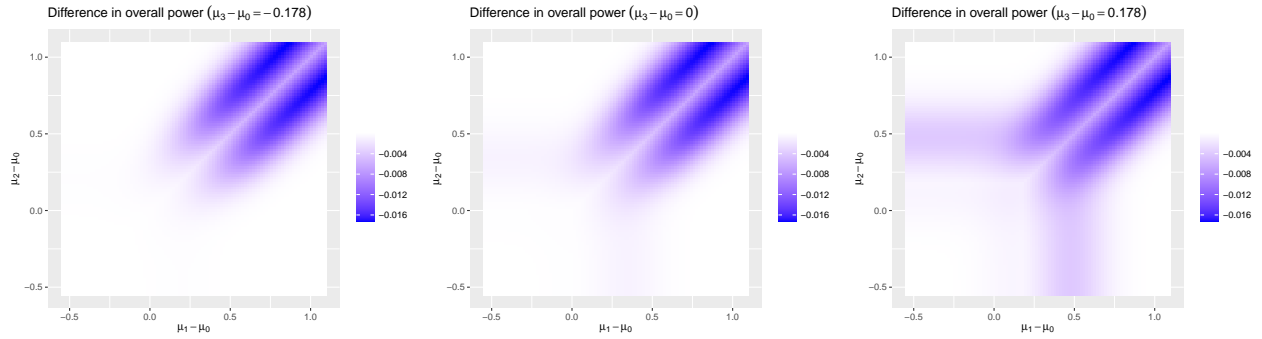

Figure 6: For multiple values of  $\mu_3 - \mu_0$ : the difference in overall power between keeping the data pre change and not.

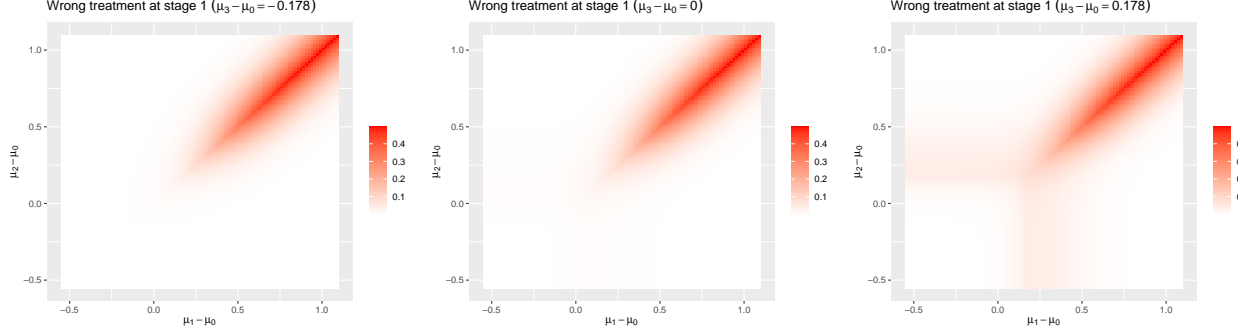

Figure 7: For multiple values of  $\mu_3 - \mu_0$ : the probability of the treatment which does not have the greatest treatment effect becoming the control at the first stage.

## 5 The effect of different values of $Z_{(1,0),1}$ and $Z_{(2,0),1}$ on the conditional power for given $\mu_1$ and $\mu_2$

Figure 8 shows the effect on conditional power for treatment 2 given treatment 1 became the control after the first stage, for different possible values of  $Z_{(1,0),1}$  and  $Z_{(2,0),1}$  given that  $\mu_1 = -0.25$  and  $\mu_2 = 0.75$ . The grey area are the values of  $Z_{(1,0),1}$  and  $Z_{(2,0),1}$  which are not possible as  $Z_{(1,0),1} < Z_{(2,0),1}$ . One only needs to consider values of  $Z_{(1,0),1} > u_1$  as otherwise treatment 1 would not be the new control. It is shown here that even in a case where on average there is very little benefit in only retaining the new information there are potential values of  $Z_{(1,0),1}$  and  $Z_{(2,0),1}$  where there is large benefit in only using the new data. For example if  $Z_{(1,0),1} = 4$  and  $Z_{(2,0),1} = 1.5$  then there is an loss in conditional power of 82.7% by retaining the old data.

## 6 Three stage conditional power given change after the first stage

The only conditional power where one may see benefit in keeping the old data in a 3 stage case when  $u_j > 0$  for all  $j$  is if the control changes at the first stage. The denominator of the conditional power for a change after the first stage is:

$$P(E_{k^*,k',1}^1 \cap E_{k^*,k',1}^2 \cap E_{k^*,k',1}^3) = \int_{u_1}^{\infty} \int_{l_1}^{\infty} \int_{-\infty}^0 \int_{-\infty}^0 \phi \left[ \mathbf{z}, \mu_{[1,2,3,4]}^{\Omega_{k^*,k',1}}, \Sigma_{[1,2,3,4]}^{\Omega_{k^*,k',1}} \right] d\mathbf{z},$$

where  $\phi(\mathbf{z}, \mu, \Sigma)$  is the probability density function of a multi-variate normal distribution with mean  $\mu$  and covariance matrix  $\Sigma$ . Also

$$\mu^{\Omega_{k^*,k',1}} = \left( \frac{\sqrt{n}(\mu_{k'} - \mu_0)}{\sigma\sqrt{2}}, \frac{\sqrt{n}(\mu_{k^*} - \mu_0)}{\sigma\sqrt{2}}, \frac{\sqrt{n}(\mu_{k^*} - \mu_{k'})}{\sigma\sqrt{2}}, \frac{\sqrt{n}(\mu_k - \mu_{k'})}{\sigma\sqrt{2}}, \frac{\sqrt{n}(\mu_{k^*} - \mu_{k'})}{\sigma}, \frac{\sqrt{3n}(\mu_{k'} - \mu_0)}{\sigma\sqrt{2}} \right)$$

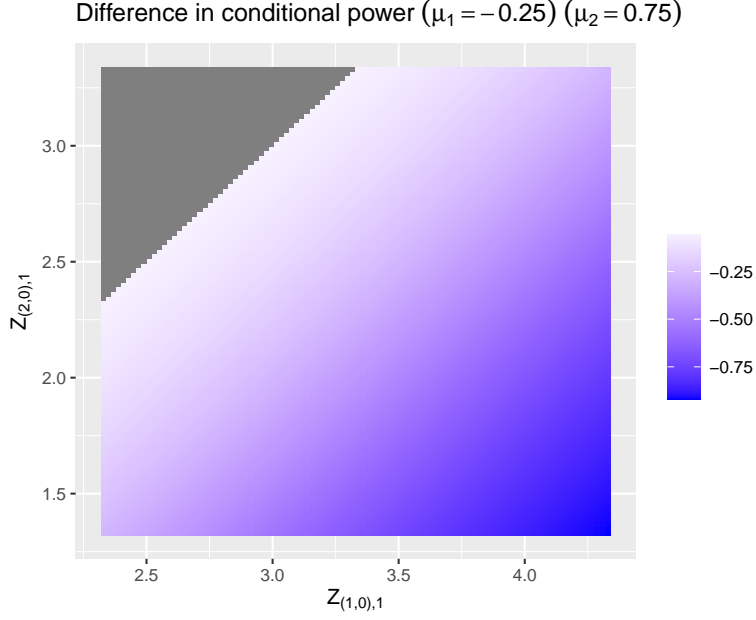

Figure 8: The difference in conditional power based on the value of the test statistics for treatment 2 given that treatment 1 has gone forward at the first stage for fixed  $\mu_1 = 0.25$  and  $\mu_2 = 0.75$ .

, and

$$\Sigma^{\Omega_{k^*,k',1}} = \begin{pmatrix} 1 & \frac{1}{2} & -\frac{1}{2} & -\frac{1}{2} & -\frac{1}{2}\sqrt{\frac{1}{2}} & -\frac{1}{2}\sqrt{\frac{1}{3}} \\ \frac{1}{2} & 1 & \frac{1}{2} & 0 & \frac{1}{2}\sqrt{\frac{1}{2}} & \frac{1}{2}\sqrt{\frac{1}{3}} \\ -\frac{1}{2} & \frac{1}{2} & 1 & \frac{1}{2} & \sqrt{\frac{1}{2}} & \sqrt{\frac{1}{3}} \\ -\frac{1}{2} & 0 & \frac{1}{2} & 1 & \frac{1}{2}\sqrt{\frac{1}{2}} & \frac{1}{2}\sqrt{\frac{1}{3}} \\ -\frac{1}{2}\sqrt{\frac{1}{2}} & \frac{1}{2}\sqrt{\frac{1}{2}} & \sqrt{\frac{1}{2}} & \frac{1}{2}\sqrt{\frac{1}{2}} & 1 & \sqrt{\frac{2}{3}} \\ -\frac{1}{2}\sqrt{\frac{1}{3}} & \frac{1}{2}\sqrt{\frac{1}{3}} & \sqrt{\frac{1}{3}} & \frac{1}{2}\sqrt{\frac{1}{3}} & \sqrt{\frac{2}{3}} & 1 \end{pmatrix}.$$

The numerator of the conditional power for a change after the first stage is:

$$\begin{aligned} P(E_{k^*,k',1}^1 \cap E_{k^*,k',1}^2 \cap E_{k^*,k',1}^3 \cap E_{k^*,k',1}^4) &= \int_{u_1}^{\infty} \int_{l_1}^{\infty} \int_{-\infty}^0 \int_{-\infty}^0 \int_{u_2}^{\infty} \phi \left[ \mathbf{z}, \mu_{[1,2,3,4,5]}^{\Omega_{k^*,k',1}}, \Sigma_{[1,2,3,4,5]}^{\Omega_{k^*,k',1}} \right] \mathbf{dz} \\ &+ \int_{u_1}^{\infty} \int_{l_1}^{\infty} \int_{-\infty}^0 \int_{-\infty}^0 \int_{l_2}^{u_2} \int_{u_3}^{\infty} \phi \left[ \mathbf{z}, \mu^{\Omega_{k^*,k',1}}, \Sigma^{\Omega_{k^*,k',1}} \right] \mathbf{dz}. \end{aligned}$$

The conditional power for treatment  $k^*$  when treatment  $k'$  becomes the new control at stage 1 is:

$$\frac{P(E_{k^*,k',1}^1 \cap E_{k^*,k',1}^2 \cap E_{k^*,k',1}^3 \cap E_{k^*,k',1}^4)}{P(E_{k^*,k',1}^1 \cap E_{k^*,k',1}^2 \cap E_{k^*,k',1}^3)}.$$

When we only retain the new information the conditional power is:

$$P(E_{k^*,k',1}^{*4}) = \int_{u_2}^{\infty} \phi \left[ \mathbf{z}, \left( \frac{\sqrt{n}(\mu_{k^*} - \mu_{k'})}{\sigma\sqrt{2}} \right), 1 \right] \mathbf{dz}.$$

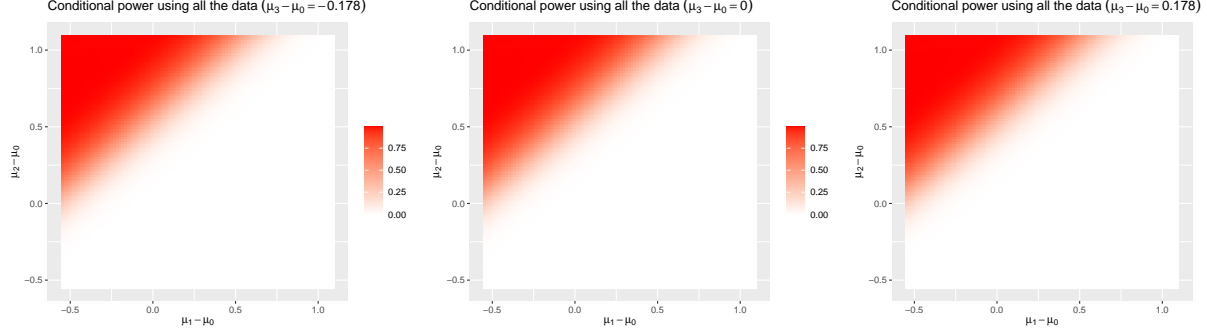

Figure 9: For multiple values of  $\mu_3 - \mu_0$  for the 3 stage example: the conditional power for treatment 2 given that treatment 1 has gone forward at the first stage when all the data is retained.

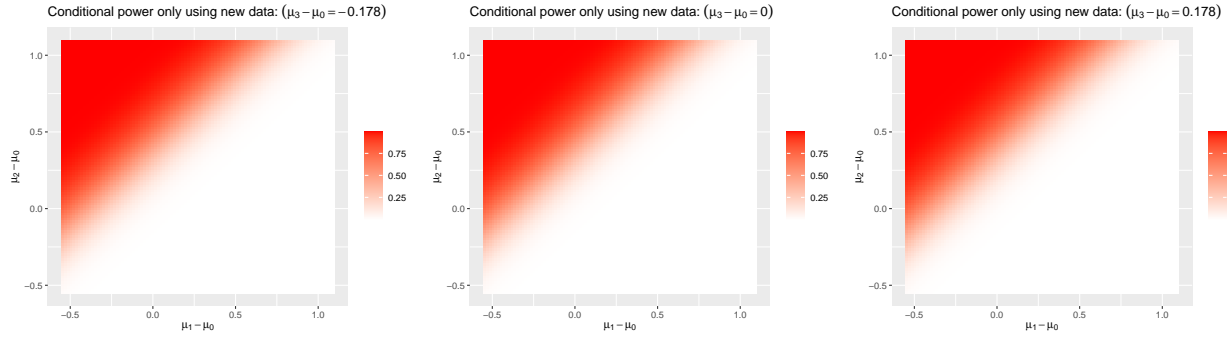

Figure 10: For multiple values of  $\mu_3 - \mu_0$  for the 3 stage example: the conditional power for treatment 2 given that treatment 1 has gone forward at the first stage when only the new data is retained.

The effect of using all the data; the post change data and the difference for conditional power between keeping the old data and not for the O'Brien and Fleming bounds (O'Brien and Fleming, 1979) are given in Figure 9, 10 and 11 respectively. The O'Brien and Fleming bounds are  $u_1 = 3.640, u_2 = 2.574, u_3 = 2.101$  and  $l_1 = -3.640, l_2 = -2.574, l_3 = 2.101$  found using the (Magirr et al., 2012). The maximum sample size using Greenstreet et al. (2023) is 312 which is based on 26 patients per stage per arm.

As can be seen even when using the negative bounds given by O'Brien and Fleming there is no advantage to keeping the old data in this example. This means that in this case for the overall power there is also no benefit to retaining the old data. However in the Supplementary Materials Section 7 we study a 3 stage example where there is benefit in keeping the old data when there are negative bounds.

## 7 Example where negative bounds can cause loss in power when only keeping new data

Consider a three stage example with  $n_1 = 100, n_2 = 101$  and  $n_3 = 10000$  and the lower bounds  $l_1 = l_2 = -1.1$  and  $u_1 = u_2 = u_3 = 2$ . We set  $\mu_1 = 1000, \mu_2 = 1000.3, \mu_3 = \mu_0 = 0$ . Then



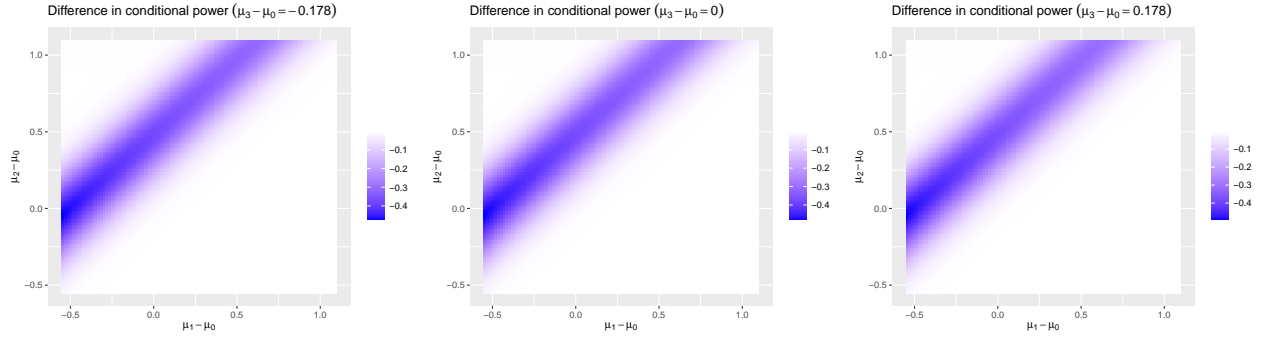

Figure 11: For multiple values of  $\mu_3 - \mu_0$  for the 3 stage example: the difference in conditional power between keeping the data pre change and not.

similar to as done above we focus on the conditional power of treatment 2 given treatment 1 has gone forward at the first stage. The conditional power is 96.4% when data is retained compared to 90.5% when only the new data is retained. This is because after the first stage there is a 9.47% chance that treatment 2 is dropped compared to treatment 1 when only the new data is used. However when old data is kept this drops to 3.63%. This therefore makes it more likely that treatment 2 will get to the final stage where there is a very high chance it will now be found superior to the control.

However even for this example if one changes the difference of  $\mu_1 - \mu_2$  then one will likely find that keeping the old data is worst than not. This section highlights that it is possible when there are negative bounds that keeping the old data can be positive, however this may not be very likely. As one can show that the conditional power difference can be positive for keeping the data, this means that this also holds for the overall power.

## 8 Simple random allocation effect on conditional power

We use a simple random allocation method to study the effect on conditional power. We simulate 100,000,000 runs of the case where treatment 1 has been taken forward after the first stage and treatment 2 is the treatment of interest. It is assumed that  $\mu_3 - \mu_0 = 0$  for the example and the triangular boundaries are used as defined in Section 5. The results of 3 different cases are given in Table 1. As can be seen in Table 1 when  $\mu_1 - \mu_0 = 0.178$  and  $\mu_2 - \mu_0 = 0.545$  the conditional power is still a lot higher when using only the data post change in control. Furthermore for this example there was only 167 simulations that found keeping all the data resulted in treatment 2 being found superior, when it was not found superior when using only the new data. This is compared to 26165252 for the other way round. This has highlighted that the conditional power and therefore overall power is still likely less when all the data is retained even when using a simple random allocation method.

Table 1: The conditional power when using a simple random allocation

| Treatment effects |                 | Conditional power |          | Treatment 2 only goes forward |               |
|-------------------|-----------------|-------------------|----------|-------------------------------|---------------|
| $\mu_1 = \mu_0$   | $\mu_2 = \mu_0$ | new data          | all data | with new data                 | with all data |
| 0.545             | 1.090           | 61.21%            | 19.37%   | 41832417                      | 649           |
| 0.545             | 0.723           | 8.26%             | 0.39%    | 7870200                       | 18            |
| 0.178             | 0.545           | 30.01%            | 3.84%    | 26165252                      | 167           |

## 9 Case 2: complete equations for calculating conditional and overall power

### 9.0.1 Conditional power equation when an arm is added later

The conditional power for treatment 1 or 2 given the other has become the control at the first stage is calculated as follows:

$$P(E_{k^*,k',1}^1 \cap E_{k^*,k',1}^2 \cap E_{k^*,k',1}^3) = \int_{u_1}^{\infty} \int_{l_1}^{\infty} \int_{-\infty}^0 \phi \left[ \mathbf{z}, \mu_{[1,2,3]}^{\Omega_{k^*,k',1}}, \Sigma_{[1,2,3]}^{\Omega_{k^*,k',1}} \right] \mathbf{dz},$$

and

$$P(E_{k^*,k',1}^1 \cap E_{k^*,k',1}^2 \cap E_{k^*,k',1}^3 \cap E_{k^*,k',1}^4) = \int_{u_1}^{\infty} \int_{l_1}^{\infty} \int_{-\infty}^0 \int_{u_2}^{\infty} \phi \left[ \mathbf{z}, \mu^{\Omega_{k^*,k',1}}, \Sigma^{\Omega_{k^*,k',1}} \right] \mathbf{dz},$$

where

$$\mu^{\Omega_{k^*,k',1}} = \left( \frac{\sqrt{n}(\mu_{k'} - \mu_0)}{\sigma\sqrt{2}}, \frac{\sqrt{n}(\mu_{k^*} - \mu_0)}{\sigma\sqrt{2}}, \frac{\sqrt{n}(\mu_{k^*} - \mu_{k'})}{\sigma\sqrt{2}}, \frac{\sqrt{n}(\mu_{k^*} - \mu_{k'})}{\sigma} \right),$$

and

$$\Sigma^{\Omega_{k^*,k',1}} = \begin{pmatrix} 1 & \frac{1}{2} & -\frac{1}{2} & -\frac{1}{2}\sqrt{\frac{1}{2}} \\ \frac{1}{2} & 1 & \frac{1}{2} & \frac{1}{2}\sqrt{\frac{1}{2}} \\ -\frac{1}{2} & \frac{1}{2} & 1 & \sqrt{\frac{1}{2}} \\ -\frac{1}{2}\sqrt{\frac{1}{2}} & \frac{1}{2}\sqrt{\frac{1}{2}} & \sqrt{\frac{1}{2}} & 1 \end{pmatrix}.$$

When only new data is kept the conditional power is:

$$P(E_{k^*,k',1}^{*4}) = \int_{u_2}^{\infty} \phi \left[ \mathbf{z}, \left( \frac{\sqrt{n}(\mu_{k^*} - \mu_{k'})}{\sigma\sqrt{2}} \right), 1 \right] \mathbf{dz}.$$

The conditional power for treatment 3 given that either treatment 1 or 2 has become the new control at their first stage is calculated as follows.

$$P(E_{k^*,k',1}^1 \cap E_{k^*,k',1}^2 \cap E_{k^*,k',1}^3 \cap E_{k^*,k',1}^4) = P(E_{k^*,k',1}^1 \cap E_{k^*,k',1}^2 \cap E_{k^*,k',1}^3) P(E_{k^*,k',1}^4),$$

where  $P(E_{k^*,k',1}^1 \cap E_{k^*,k',1}^2 \cap E_{k^*,k',1}^3)$  is equals

$$P(E_{k^*,k',1}^1 \cap E_{k^*,k',1}^2 \cap E_{k^*,k',1}^3) = \int_{u_1}^{\infty} \int_{-\infty}^0 \phi \left[ \mathbf{z}, \left( \frac{\sqrt{n}(\mu_{k'} - \mu_0)}{\sigma\sqrt{2}}, \frac{\sqrt{n}(\mu_{k^*} - \mu_{k'})}{\sigma\sqrt{2}} \right), \begin{pmatrix} 1 & -\frac{1}{2} \\ -\frac{1}{2} & 1 \end{pmatrix} \right] \mathbf{dz},$$

and  $P(E_{k^*,k',1}^4)$  is

$$P(E_{k^*,k',1}^4) = \int_{u_1}^{\infty} \phi \left[ \mathbf{z}, \left( \frac{\sqrt{n}(\mu_{k^*} - \mu_{k'})}{\sigma\sqrt{2}} \right), 1 \right] \mathbf{dz} + \int_{l_1}^{u_1} \int_{u_2}^{\infty} \phi \left[ \mathbf{z}, \left( \frac{\sqrt{n}(\mu_{k^*} - \mu_{k'})}{\sigma\sqrt{2}}, \frac{\sqrt{n}(\mu_{k^*} - \mu_{k'})}{\sigma} \right), \begin{pmatrix} 1 & \sqrt{\frac{1}{2}} \\ \sqrt{\frac{1}{2}} & 1 \end{pmatrix} \right] \mathbf{dz}.$$

Therefore the conditional power for both when old concurrent data is used and only new concurrent data is used is  $P(E_{k^*,k',1}^4)$ .

When treatment 1 or treatment 2 becomes the control at there second stage the conditional power is as follows, where we define treatment  $k_1 = \{1, 2\}/k'$  for the other treatment tested which did not become the control.

$$P(E_{k^*,k',2}^1 \cap E_{k^*,k',2}^2 \cap E_{k^*,k',2}^3) = \int_{l_1}^{u_1} \int_{u_2}^{\infty} \int_{l_1}^{u_1} \int_{-\infty}^{l_1} \phi \left[ \mathbf{z}, \mu_{[1,2,3,5]}^{\Omega_{k^*,k',2}}, \Sigma_{[1,2,3,5]}^{\Omega_{k^*,k',2}} \right] \mathbf{dz} + \int_{l_1}^{u_1} \int_{u_2}^{\infty} \int_{l_1}^{u_1} \int_{l_1}^{u_1} \int_{-\infty}^0 \phi \left[ \mathbf{z}, \mu_{[1,2,3,5,6]}^{\Omega_{k^*,k',2}}, \Sigma_{[1,2,3,5,6]}^{\Omega_{k^*,k',2}} \right] \mathbf{dz} + \int_{l_1}^{u_1} \int_{u_2}^{\infty} \int_{u_1}^{\infty} \int_{-\infty}^0 \int_{-\infty}^{l_1} \phi \left[ \mathbf{z}, \mu_{[1,2,3,4,5]}^{\Omega_{k^*,k',2}}, \Sigma_{[1,2,3,4,5]}^{\Omega_{k^*,k',2}} \right] \mathbf{dz} + \int_{l_1}^{u_1} \int_{u_2}^{\infty} \int_{u_1}^{\infty} \int_{-\infty}^0 \int_{l_1}^{u_1} \int_{-\infty}^0 \phi \left[ \mathbf{z}, \mu_{[1,2,3,4,5,6]}^{\Omega_{k^*,k',2}}, \Sigma_{[1,2,3,4,5,6]}^{\Omega_{k^*,k',2}} \right] \mathbf{dz},$$

and

$$\Omega_{k^*,k',2} = P(E_{k^*,k',2}^1 \cap E_{k^*,k',2}^2 \cap E_{k^*,k',2}^3 \cap E_{k^*,k',2}^4) = \int_{l_1}^{u_1} \int_{u_2}^{\infty} \int_{l_1}^{u_1} \int_{-\infty}^{l_1} \int_{u_2}^{\infty} \phi \left[ \mathbf{z}, \mu_{[1,2,3,5,7]}^{\Omega_{k^*,k',2}}, \Sigma_{[1,2,3,5,7]}^{\Omega_{k^*,k',2}} \right] \mathbf{dz} + \int_{l_1}^{u_1} \int_{u_2}^{\infty} \int_{l_1}^{u_1} \int_{l_1}^{u_1} \int_{-\infty}^0 \int_{u_2}^{\infty} \phi \left[ \mathbf{z}, \mu_{[1,2,3,5,6,7]}^{\Omega_{k^*,k',2}}, \Sigma_{[1,2,3,5,6,7]}^{\Omega_{k^*,k',2}} \right] \mathbf{dz} + \int_{l_1}^{u_1} \int_{u_2}^{\infty} \int_{u_1}^{\infty} \int_{-\infty}^0 \int_{-\infty}^{l_1} \int_{u_2}^{\infty} \phi \left[ \mathbf{z}, \mu_{[1,2,3,4,5,7]}^{\Omega_{k^*,k',2}}, \Sigma_{[1,2,3,4,5,7]}^{\Omega_{k^*,k',2}} \right] \mathbf{dz} + \int_{l_1}^{u_1} \int_{u_2}^{\infty} \int_{u_1}^{\infty} \int_{-\infty}^0 \int_{l_1}^{u_1} \int_{-\infty}^0 \int_{u_2}^{\infty} \phi \left[ \mathbf{z}, \mu_{[1,2,3,4,5,6,7]}^{\Omega_{k^*,k',2}}, \Sigma_{[1,2,3,4,5,6,7]}^{\Omega_{k^*,k',2}} \right] \mathbf{dz},$$

where

$$\mu^{\Omega_{k^*,k',2}} = \left( \frac{\sqrt{n}(\mu_{k'} - \mu_0)}{\sigma\sqrt{2}}, \frac{\sqrt{n}(\mu_{k'} - \mu_0)}{\sigma}, \frac{\sqrt{n}(\mu_{k^*} - \mu_0)}{\sigma\sqrt{2}}, \frac{\sqrt{n}(\mu_{k^*} - \mu_{k'})}{\sigma\sqrt{2}}, \frac{\sqrt{n}(\mu_{k_1} - \mu_0)}{\sigma\sqrt{2}}, \frac{\sqrt{n}(\mu_{k_1} - \mu_{k'})}{\sigma}, \frac{\sqrt{n}(\mu_{k^*} - \mu_{k'})}{\sigma} \right),$$

and

$$\Sigma^{\Omega_{k^*,k',2}} = \begin{pmatrix} 1 & \sqrt{\frac{1}{2}} & 0 & 0 & \frac{1}{2} & -\frac{1}{2}\sqrt{\frac{1}{2}} & 0 \\ \sqrt{\frac{1}{2}} & 1 & \frac{1}{2}\sqrt{\frac{1}{2}} & -\frac{1}{2}\sqrt{\frac{1}{2}} & \frac{1}{2}\sqrt{\frac{1}{2}} & -\frac{1}{2} & -\frac{1}{4} \\ 0 & \frac{1}{2}\sqrt{\frac{1}{2}} & 1 & \frac{1}{2} & 0 & 0 & \frac{1}{2}\sqrt{\frac{1}{2}} \\ 0 & -\frac{1}{2}\sqrt{\frac{1}{2}} & \frac{1}{2} & 1 & 0 & \frac{1}{2}\sqrt{\frac{1}{2}} & \sqrt{\frac{1}{2}} \\ \frac{1}{2} & \frac{1}{2}\sqrt{\frac{1}{2}} & 0 & 0 & 1 & \frac{1}{2}\sqrt{\frac{1}{2}} & 0 \\ -\frac{1}{2}\sqrt{\frac{1}{2}} & -\frac{1}{2} & 0 & \frac{1}{2}\sqrt{\frac{1}{2}} & \frac{1}{2}\sqrt{\frac{1}{2}} & 1 & \frac{1}{4} \\ 0 & -\frac{1}{4} & \frac{1}{2}\sqrt{\frac{1}{2}} & \sqrt{\frac{1}{2}} & 0 & \frac{1}{4} & 1 \end{pmatrix}.$$

The conditional power when only using new data is

$$P(E_{k^*,k',1}^{*4}) = \int_{u_2}^{\infty} \phi \left[ \mathbf{z}, \left( \frac{\sqrt{n}(\mu_{k^*} - \mu_{k'})}{\sigma\sqrt{2}} \right), 1 \right] \mathbf{dz}.$$

### 9.0.2 Overall power

When studying the overall power if the treatment with the greatest effect starts at the beginning of the trial we define,  $k_1$  be the other treatment that starts the trial at the beginning, and let  $k_2$  be the treatment which starts after the first stage. Then the probability treatment  $k^*$  becomes the new control at the first stage is:

$$\Xi_{k,1} = \int_{u_1}^{\infty} \int_{-\infty}^0 \phi \left[ \mathbf{z}, \mu^{\Xi_{k,1}}, \Sigma^{\Xi_{k,1}} \right] \mathbf{dz},$$

where

$$\Sigma^{\Xi_{k,1}} = \begin{pmatrix} 1 & -\frac{1}{2} \\ -\frac{1}{2} & 1 \end{pmatrix},$$

and

$$\mu^{\Xi_{k,1}} = \left( \frac{\sqrt{n}(\mu_{k^*} - \mu_0)}{\sigma\sqrt{2}}, \frac{\sqrt{n}(\mu_{k_1} - \mu_{k^*})}{\sigma\sqrt{2}} \right).$$

The probability treatment  $k^*$  becomes the new control at the second stage is:

$$\begin{aligned} \Xi_{k,2} = & \int_{l_1}^{u_1} \int_{u_2}^{\infty} \int_{-\infty}^{l_1} \int_{-\infty}^{u_1} \phi \left[ \mathbf{z}, \mu_{[1,2,3,5]}^{\Xi_{k,2}}, \Sigma_{[1,2,3,5]}^{\Xi_{k,2}} \right] \mathbf{dz} \\ & + \int_{l_1}^{u_1} \int_{u_2}^{\infty} \int_{l_1}^{u_1} \int_{-\infty}^0 \int_{-\infty}^{u_1} \phi \left[ \mathbf{z}, \mu_{[1,2,3,4,5]}^{\Xi_{k,2}}, \Sigma_{[1,2,3,4,5]}^{\Xi_{k,2}} \right] \mathbf{dz} \\ & + \int_{l_1}^{u_1} \int_{u_2}^{\infty} \int_{-\infty}^{l_1} \int_{u_1}^{\infty} \int_{-\infty}^0 \phi \left[ \mathbf{z}, \mu_{[1,2,3,5,6]}^{\Xi_{k,2}}, \Sigma_{[1,2,3,5,6]}^{\Xi_{k,2}} \right] \mathbf{dz} + \\ & \int_{l_1}^{u_1} \int_{u_2}^{\infty} \int_{l_1}^{u_1} \int_{-\infty}^0 \int_{u_1}^{\infty} \int_{-\infty}^0 \phi \left[ \mathbf{z}, \mu^{\Xi_{k,2}}, \Sigma^{\Xi_{k,2}} \right] \mathbf{dz}, \end{aligned}$$

where

$$\Sigma^{\Xi_{k,2}} = \begin{pmatrix} 1 & \sqrt{\frac{1}{2}} & \frac{1}{2} & -\frac{1}{2}\sqrt{\frac{1}{2}} & 0 & 0 \\ \sqrt{\frac{1}{2}} & 1 & \frac{1}{2}\sqrt{\frac{1}{2}} & -\frac{1}{2} & \frac{1}{2}\sqrt{\frac{1}{2}} & -\frac{1}{2}\sqrt{\frac{1}{2}} \\ \frac{1}{2} & \frac{1}{2}\sqrt{\frac{1}{2}} & 1 & \frac{1}{2}\sqrt{\frac{1}{2}} & \frac{1}{2} & 0 \\ -\frac{1}{2}\sqrt{\frac{1}{2}} & -\frac{1}{2} & \frac{1}{2}\sqrt{\frac{1}{2}} & 1 & 0 & \frac{1}{2}\sqrt{\frac{1}{2}} \\ 0 & \frac{1}{2}\sqrt{\frac{1}{2}} & 0 & 0 & 1 & \frac{1}{2} \\ 0 & \frac{1}{2}\sqrt{\frac{1}{2}} & 0 & \frac{1}{2}\sqrt{\frac{1}{2}} & \frac{1}{2} & 1 \end{pmatrix},$$

and

$$\mu^{\Xi_{k,2}} = \left( \frac{\sqrt{n}(\mu_{k^*} - \mu_0)}{\sigma\sqrt{2}}, \frac{\sqrt{n}(\mu_{k^*} - \mu_0)}{\sigma}, \frac{\sqrt{n}(\mu_{k_1} - \mu_0)}{\sigma\sqrt{2}}, \frac{\sqrt{n}(\mu_{k_1} - \mu_{k^*})}{\sigma}, \right. \\ \left. \frac{\sqrt{n}(\mu_{k_2} - \mu_0)}{\sigma\sqrt{2}}, \frac{\sqrt{n}(\mu_{k_2} - \mu_{k^*})}{\sigma\sqrt{2}} \right).$$

Therefore the overall power for treatment  $k^*$  given it starts the trial at the start is

$$\sum_{j^*=1}^2 \Xi_{k^*,j^*} + \Omega_{k^*,k'=\{1,2\}/k^*,1}.$$

Now we consider when  $k^*$  is the treatment which is added later (i.e treatment 3). Now  $k_1$  and  $k_2$  are both for the treatments which began the trial. The probability treatment  $k^*$  becomes the new control at its first stage is:

$$\begin{aligned} \Xi_{k,1} = & \int_{u_1}^{\infty} \int_{-\infty}^{l_1} \int_{-\infty}^{l_1} \phi \left[ \mathbf{z}, \mu_{[1,2,5]}^{\Xi_{k,1}}, \Sigma_{[1,2,5]}^{\Xi_{k,1}} \right] \mathbf{dz} + \int_{u_1}^{\infty} \int_{-\infty}^{l_1} \int_{l_1}^{u_1} \int_{-\infty}^{u_2} \phi \left[ \mathbf{z}, \mu_{[1,2,5,6]}^{\Xi_{k,1}}, \Sigma_{[1,2,5,6]}^{\Xi_{k,1}} \right] \mathbf{dz} + \\ & \int_{u_1}^{\infty} \int_{-\infty}^{l_1} \int_{l_1}^{u_1} \int_{u_2}^{\infty} \int_{-\infty}^0 \phi \left[ \mathbf{z}, \mu_{[1,2,5,6,7]}^{\Xi_{k,1}}, \Sigma_{[1,2,5,6,7]}^{\Xi_{k,1}} \right] \mathbf{dz} + \int_{u_1}^{\infty} \int_{l_1}^{u_1} \int_{-\infty}^{u_2} \int_{-\infty}^{l_1} \phi \left[ \mathbf{z}, \mu_{[1,2,3,5]}^{\Xi_{k,1}}, \right. \\ & \left. \Sigma_{[1,2,3,5]}^{\Xi_{k,1}} \right] \mathbf{dz} + \int_{u_1}^{\infty} \int_{l_1}^{u_1} \int_{-\infty}^{u_2} \int_{l_1}^{u_1} \int_{-\infty}^{u_2} \phi \left[ \mathbf{z}, \mu_{[1,2,3,5,6]}^{\Xi_{k,1}}, \Sigma_{[1,2,3,5,6]}^{\Xi_{k,1}} \right] \mathbf{dz} + \\ & \int_{u_1}^{\infty} \int_{l_1}^{u_1} \int_{-\infty}^{u_2} \int_{l_1}^{u_1} \int_{u_2}^{\infty} \int_{-\infty}^0 \phi \left[ \mathbf{z}, \mu_{[1,2,3,5,6,7]}^{\Xi_{k,1}}, \Sigma_{[1,2,3,5,6,7]}^{\Xi_{k,1}} \right] \mathbf{dz} + \\ & \int_{u_1}^{\infty} \int_{l_1}^{u_1} \int_{u_2}^{\infty} \int_{-\infty}^0 \int_{-\infty}^{l_1} \phi \left[ \mathbf{z}, \mu_{[1,2,3,4,5]}^{\Xi_{k,1}}, \Sigma_{[1,2,3,4,5]}^{\Xi_{k,1}} \right] \mathbf{dz} + \\ & \int_{u_1}^{\infty} \int_{l_1}^{u_1} \int_{u_2}^{\infty} \int_{-\infty}^0 \int_{l_1}^{u_1} \int_{-\infty}^{u_2} \phi \left[ \mathbf{z}, \mu_{[1,2,3,4,5,6]}^{\Xi_{k,1}}, \Sigma_{[1,2,3,4,5,6]}^{\Xi_{k,1}} \right] \mathbf{dz} + \\ & \int_{u_1}^{\infty} \int_{l_1}^{u_1} \int_{u_2}^{\infty} \int_{-\infty}^0 \int_{l_1}^{u_1} \int_{u_2}^{\infty} \int_{-\infty}^0 \phi \left[ \mathbf{z}, \mu^{\Xi_{k,1}}, \Sigma^{\Xi_{k,1}} \right] \mathbf{dz}, \end{aligned}$$

where

$$\Sigma^{\Xi_{k,1}} = \begin{pmatrix} 1 & 0 & \frac{1}{2}\sqrt{\frac{1}{2}} & -\frac{1}{2} & 0 & \frac{1}{2}\sqrt{\frac{1}{2}} & -\frac{1}{2} \\ 0 & 1 & \sqrt{\frac{1}{2}} & 0 & \frac{1}{2} & \frac{1}{2}\sqrt{\frac{1}{2}} & 0 \\ \frac{1}{2}\sqrt{\frac{1}{2}} & \sqrt{\frac{1}{2}} & 1 & \frac{1}{2}\sqrt{\frac{1}{2}} & \frac{1}{2}\sqrt{\frac{1}{2}} & \frac{1}{2} & 0 \\ -\frac{1}{2} & 0 & \frac{1}{2}\sqrt{\frac{1}{2}} & 1 & 0 & 0 & \frac{1}{2} \\ 0 & \frac{1}{2} & \frac{1}{2}\sqrt{\frac{1}{2}} & 0 & 1 & \sqrt{\frac{1}{2}} & 0 \\ \frac{1}{2}\sqrt{\frac{1}{2}} & \frac{1}{2}\sqrt{\frac{1}{2}} & \frac{1}{2} & 0 & \sqrt{\frac{1}{2}} & 1 & \frac{1}{2}\sqrt{\frac{1}{2}} \\ -\frac{1}{2} & 0 & 0 & \frac{1}{2} & 0 & \frac{1}{2}\sqrt{\frac{1}{2}} & 1 \end{pmatrix},$$

and

$$\mu^{\Xi_{k,1}} = \left( \frac{\sqrt{n}(\mu_{k^*} - \mu_0)}{\sigma\sqrt{2}}, \frac{\sqrt{n}(\mu_{k_1} - \mu_0)}{\sigma\sqrt{2}}, \frac{\sqrt{n}(\mu_{k_1} - \mu_0)}{\sigma}, \frac{\sqrt{n}(\mu_{k_1} - \mu_{k^*})}{\sigma\sqrt{2}}, \right. \\ \left. , \frac{\sqrt{n}(\mu_{k_2} - \mu_0)}{\sigma\sqrt{2}}, \frac{\sqrt{n}(\mu_{k_2} - \mu_0)}{\sigma}, \frac{\sqrt{n}(\mu_{k_2} - \mu_{k^*})}{\sigma\sqrt{2}} \right).$$

The probability treatment  $k^*$  becomes the new control at its second stage is:

$$\Xi_{k,2} = \int_{l_1}^{u_1} \int_{u_2}^{\infty} \int_{-\infty}^{l_1} \int_{-\infty}^{l_1} \phi \left[ \mathbf{z}, \mu_{[1,2,3,5]}^{\Xi_{k,2}}, \Sigma_{[1,2,3,5]}^{\Xi_{k,2}} \right] \mathbf{dz} + \int_{l_1}^{u_1} \int_{u_2}^{\infty} \int_{-\infty}^{l_1} \int_{l_1}^{u_1} \int_{-\infty}^{u_2} \phi \left[ \mathbf{z}, \mu_{[1,2,3,5,6]}^{\Xi_{k,2}}, \right. \\ \left. \Sigma_{[1,2,3,5,6]}^{\Xi_{k,2}} \right] \mathbf{dz} + \int_{l_1}^{u_1} \int_{u_2}^{\infty} \int_{l_1}^{u_1} \int_{-\infty}^{u_2} \int_{-\infty}^{l_1} \phi \left[ \mathbf{z}, \mu_{[1,2,3,4,5]}^{\Xi_{k,2}}, \Sigma_{[1,2,3,4,5]}^{\Xi_{k,2}} \right] \mathbf{dz} \\ + \int_{l_1}^{u_1} \int_{u_2}^{\infty} \int_{l_1}^{u_1} \int_{-\infty}^{u_2} \int_{l_1}^{u_1} \int_{-\infty}^{u_2} \phi \left[ \mathbf{z}, \mu^{\Xi_{k,2}}, \Sigma^{\Xi_{k,2}} \right] \mathbf{dz},$$

where

$$\Sigma^{\Xi_{k,2}} = \begin{pmatrix} 1 & \sqrt{\frac{1}{2}} & 0 & \frac{1}{2}\sqrt{\frac{1}{2}} & 0 & \frac{1}{2}\sqrt{\frac{1}{2}} \\ \sqrt{\frac{1}{2}} & 1 & 0 & \frac{1}{4} & 0 & \frac{1}{4} \\ 0 & 0 & 1 & \sqrt{\frac{1}{2}} & \frac{1}{2} & \frac{1}{2}\sqrt{\frac{1}{2}} \\ \frac{1}{2}\sqrt{\frac{1}{2}} & \frac{1}{4} & \sqrt{\frac{1}{2}} & 1 & \frac{1}{2}\sqrt{\frac{1}{2}} & \frac{1}{2} \\ 0 & 0 & \frac{1}{2} & \frac{1}{2}\sqrt{\frac{1}{2}} & 1 & \sqrt{\frac{1}{2}} \\ \frac{1}{2}\sqrt{\frac{1}{2}} & \frac{1}{4} & \frac{1}{2}\sqrt{\frac{1}{2}} & \frac{1}{2} & \sqrt{\frac{1}{2}} & 1 \end{pmatrix},$$

and

$$\mu^{\Xi_{k,2}} = \left( \frac{\sqrt{n}(\mu_{k^*} - \mu_0)}{\sigma\sqrt{2}}, \frac{\sqrt{n}(\mu_{k^*} - \mu_0)}{\sigma}, \frac{\sqrt{n}(\mu_{k_1} - \mu_0)}{\sigma\sqrt{2}}, \frac{\sqrt{n}(\mu_{k_1} - \mu_0)}{\sigma}, \right. \\ \left. \frac{\sqrt{n}(\mu_{k_2} - \mu_0)}{\sigma\sqrt{2}}, \frac{\sqrt{n}(\mu_{k_2} - \mu_0)}{\sigma} \right).$$

Therefore, the overall power for treatment  $k^*$  given it is the treatment which is added later is:

$$\sum_{j^*=1}^2 \Xi_{k^*,j^*} + \sum_{k' \in \{1,2\}} \sum_{j'=1}^2 \Omega_{k^*,k',j'}.$$

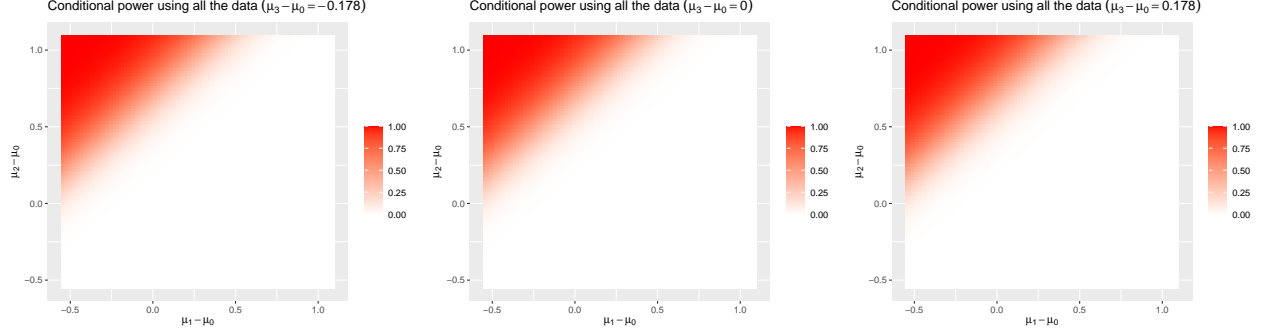

Figure 12: For multiple values of  $\mu_3 - \mu_0$  with treatment 3 added later: the conditional power for treatment 2 given that treatment 1 has gone forward at the first stage when all the data is retained.

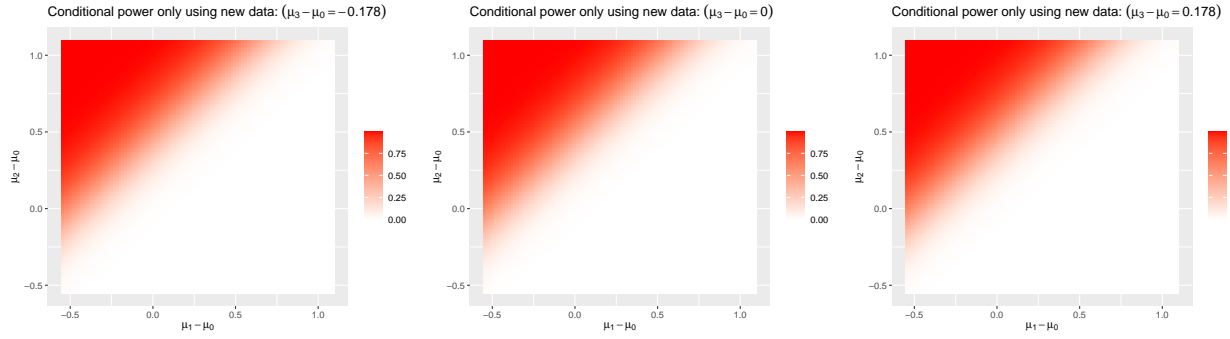

Figure 13: For multiple values of  $\mu_3 - \mu_0$  with treatment 3 added later: the conditional power for treatment 2 given that treatment 1 has gone forward at the first stage when only the data post the change in control is used.

## 10 Complete results for Case 2

### 10.0.1 Conditional power for treatment 2 against treatment 1 after the first stage

The results of using different values of  $\mu_3 - \mu_0$  are studied. The values studied are  $\mu_3 - \mu_0 = -\theta_0$ ,  $\mu_3 - \mu_0 = 0$  and  $\mu_3 - \mu_0 = \theta_0$ . The conditional power for treatment 2 given treatment 1 has become the new control at stage 1 when using all the data is given in Figure 12. The conditional power for treatment 2 given treatment 1 has become the new control at stage 1 when using only the new data is given in Figure 13. The difference in conditional power for treatment 2 given treatment 1 has become the new control at stage 1 is given in Figure 14.

### 10.0.2 Conditional power for treatment 3 against treatment 1 after the first stage

The results of using different values of  $\mu_2 - \mu_0$  are studied. The values studied are  $\mu_2 - \mu_0 = -\theta_0$ ,  $\mu_2 - \mu_0 = 0$  and  $\mu_2 - \mu_0 = \theta_0$ . The conditional power for treatment 3 given treatment 1 has become the new control at stage 1 is given in Figure 15.

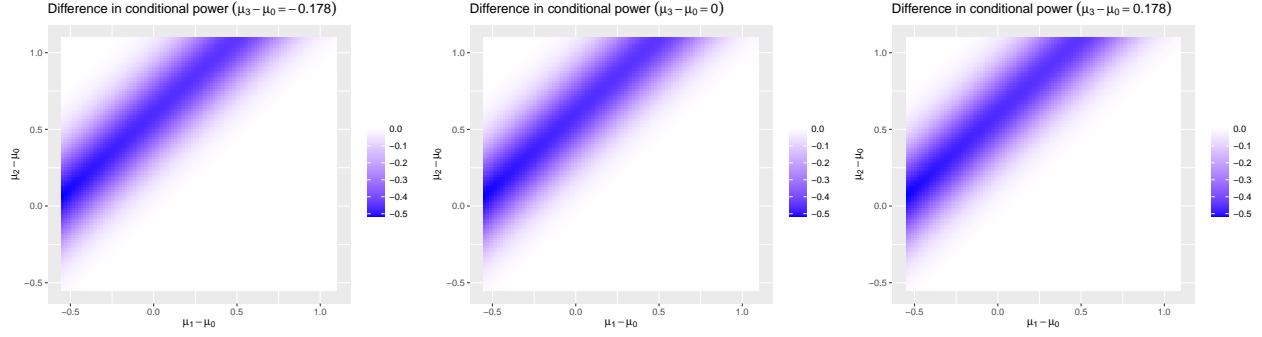

Figure 14: For multiple values of  $\mu_3 - \mu_0$  with treatment 3 added later: the difference in conditional power between keeping the data pre change and not.

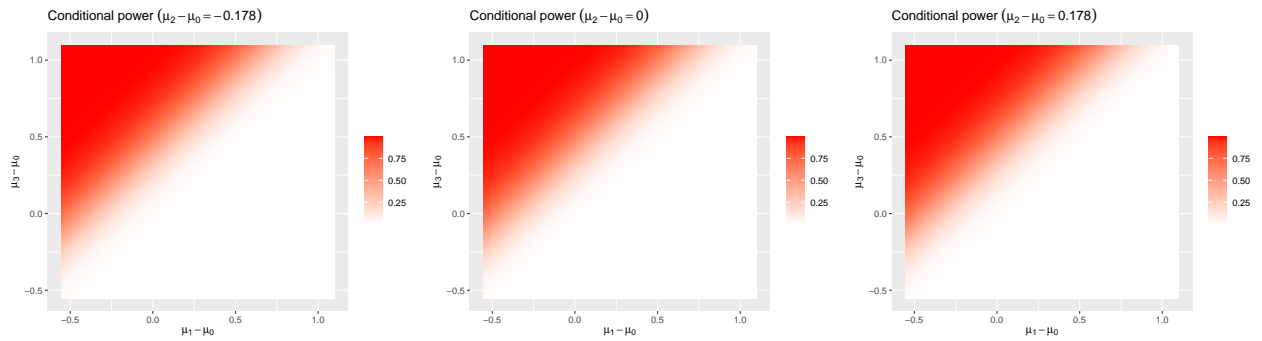

Figure 15: For multiple values of  $\mu_2 - \mu_0$  with treatment 3 added later: the conditional power for treatment 3 given that treatment 1 has gone forward at the first stage.



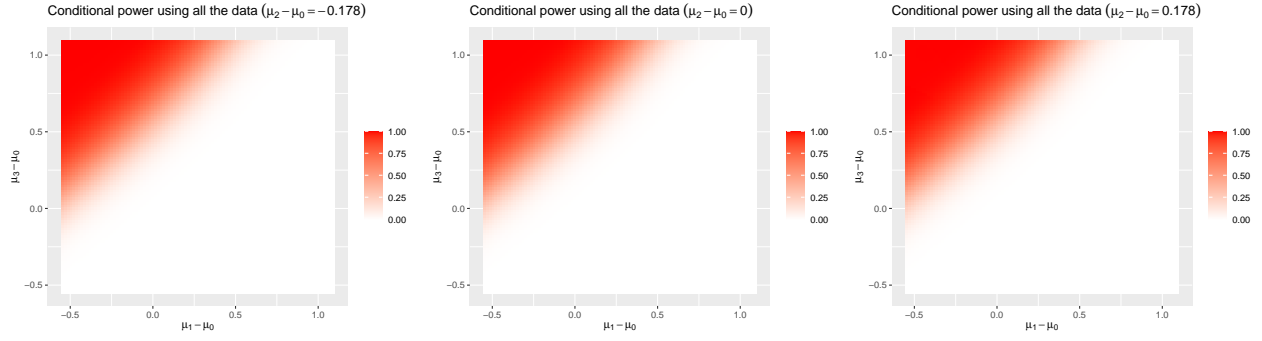

Figure 16: For multiple values of  $\mu_2 - \mu_0$  with treatment 3 added later: the conditional power for treatment 3 given that treatment 1 has gone forward at the second stage when all the data is retained.

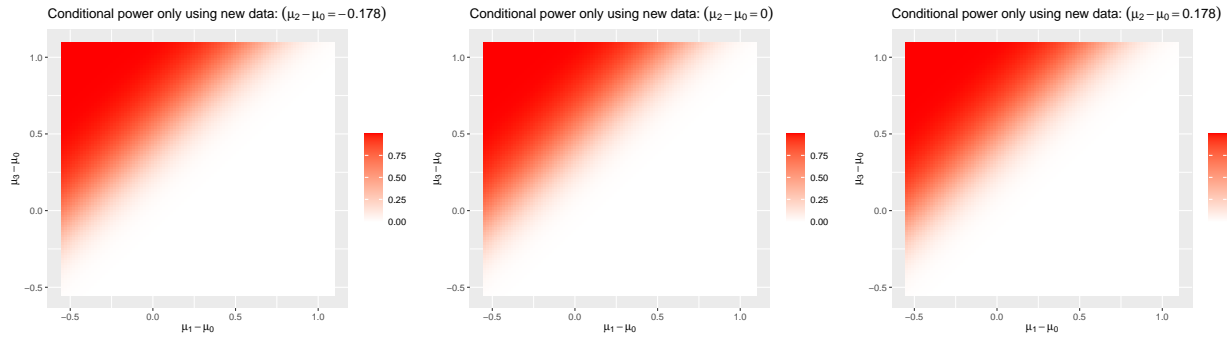

Figure 17: For multiple values of  $\mu_2 - \mu_0$  with treatment 3 added later: the conditional power for treatment 3 given that treatment 1 has gone forward at the second stage when only the data post the change in control is used.

### 10.0.3 Conditional power for treatment 3 against treatment 1 after the second stage

The results of using different values of  $\mu_2 - \mu_0$  are studied. The values studied are  $\mu_2 - \mu_0 = -\theta_0$ ,  $\mu_2 - \mu_0 = 0$  and  $\mu_2 - \mu_0 = \theta_0$ . The conditional power for treatment 3 given treatment 1 has become the new control at stage 2 when using all the data is given in Figure 16. The conditional power for treatment 3 given treatment 1 has become the new control at stage 1 when using only the new data is given in Figure 17. The difference in conditional power for treatment 3 given treatment 1 has become the new control at stage 1 is given in Figure 18.

### 10.0.4 Overall power for treatment 2 against treatment 1

The results of using different values of  $\mu_3 - \mu_0$  are studied. The values studied are  $\mu_3 - \mu_0 = -\theta_0$ ,  $\mu_3 - \mu_0 = 0$  and  $\mu_3 - \mu_0 = \theta_0$ . The overall power when using all the data is given in Figure 19. The overall power when using only the new data is given in Figure 20. The difference in overall power is given in Figure 21.

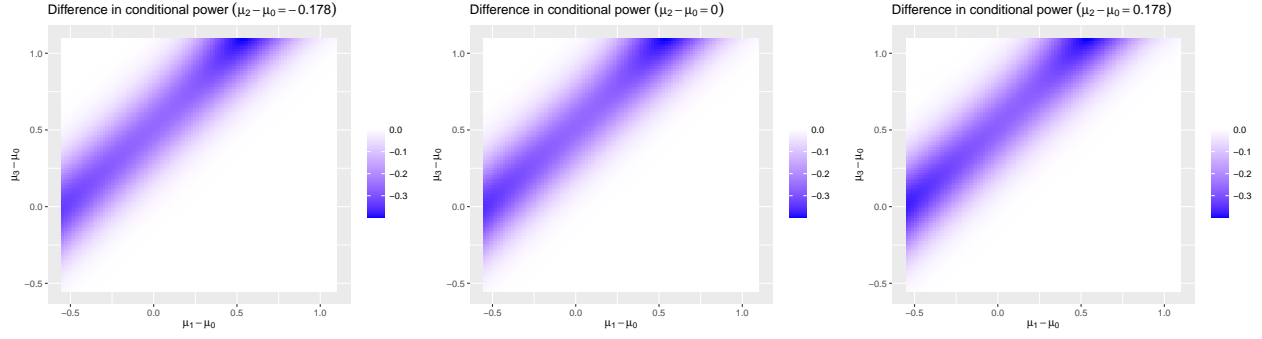

Figure 18: For multiple values of  $\mu_2 - \mu_0$  with treatment 3 added later: the difference in conditional power between keeping the data pre change and not.

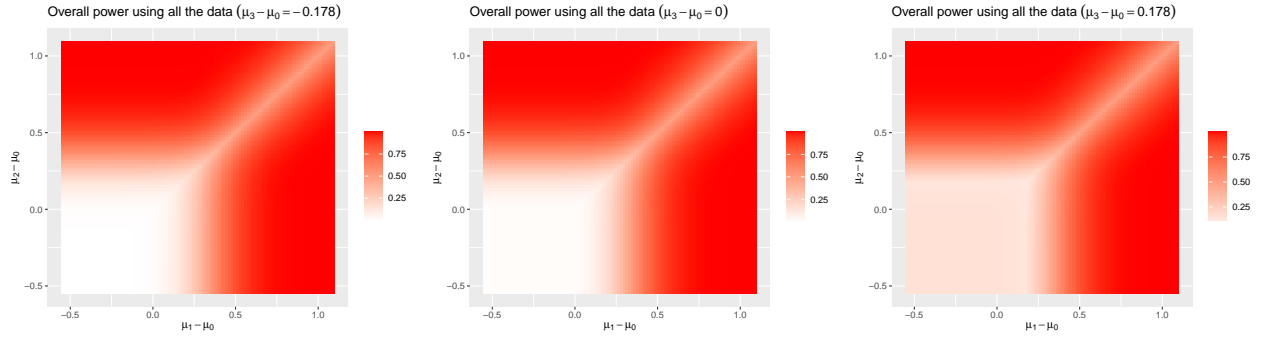

Figure 19: For multiple values of  $\mu_3 - \mu_0$  with treatment 3 added later: the overall power when all the data is retained.

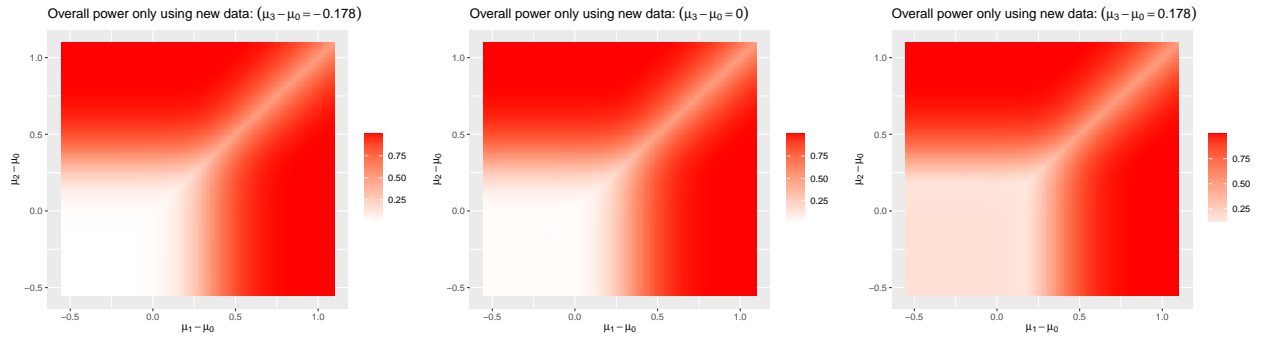

Figure 20: For multiple values of  $\mu_3 - \mu_0$  with treatment 3 added later: the overall power when only the data post the change in control is used.

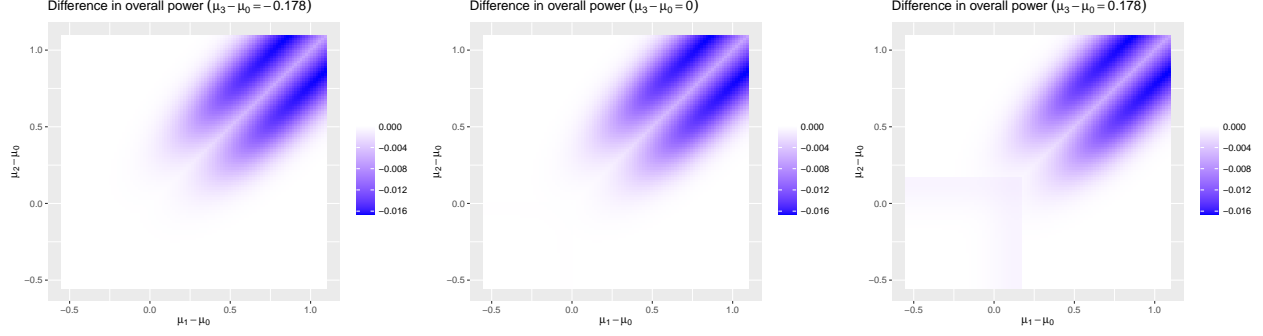

Figure 21: For multiple values of  $\mu_3 - \mu_0$  with treatment 3 added later: the difference in overall power between keeping the data pre change and not.

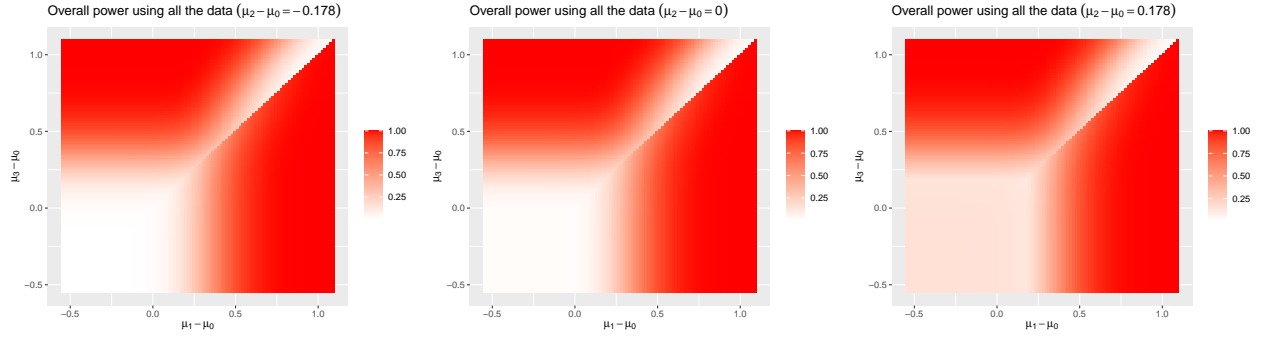

Figure 22: For multiple values of  $\mu_2 - \mu_0$  with treatment 3 added later: the overall power when all the data is retained.

### 10.0.5 Overall power for treatment 3 against treatment 1

The results of using different values of  $\mu_2 - \mu_0$  are studied. The values studied are  $\mu_2 - \mu_0 = -\theta_0$ ,  $\mu_2 - \mu_0 = 0$  and  $\mu_2 - \mu_0 = \theta_0$ . The overall power when using all the data is given in Figure 22. The overall power when using only the new data is given in Figure 23. The difference in overall power is given in Figure 24.

## 11 Added later with no interim analyses

In this example each treatment only has one analysis as is illustrated in Figure 25. Therefore when treatment 1 and 2 have their analysis treatment 3 is halfway through recruitment and is not studied at this point. The upper and lower boundaries are found using the method in Greenstreet et al. (2021) to once again control the FWER at 5%. They are  $u_1 = l_1 = 2.089$ . In addition each active treatment gets 78 patients so the maximum sample size is 351 in order to control the pairwise power at 90% (Greenstreet et al., 2023).

For the conditional power there is only one point where this is non zero and this is if either treatment 1 or 2 go forward at there final analysis with treatment 3 being the one of interest. If one assumes it was treatment 1 that goes forward the conditional power for treatment 3 if all the data is used, for multiple values of  $\mu_2 - \mu_0$ , can be seen in Figure 26. Similarly in Figure 27 the conditional power if only the data post change is used. Figure 28 shows the difference

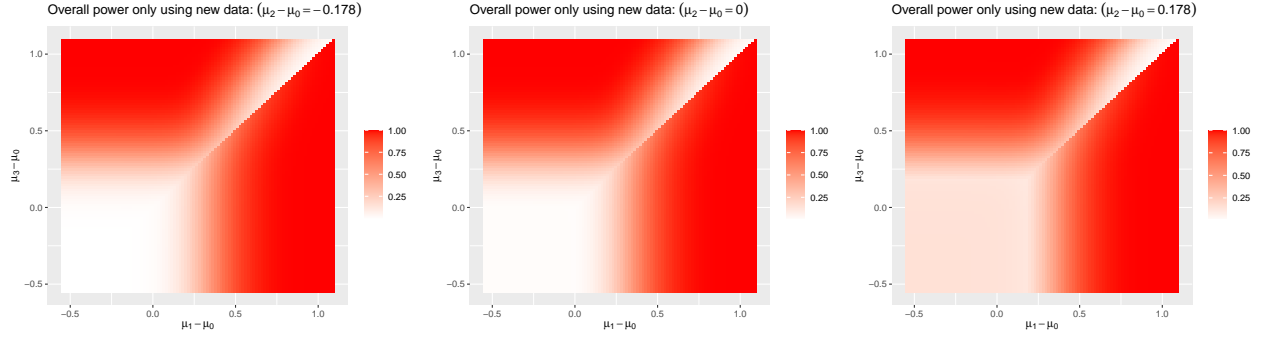

Figure 23: For multiple values of  $\mu_2 - \mu_0$  with treatment 3 added later: the overall power when only the data post the change in control is used.

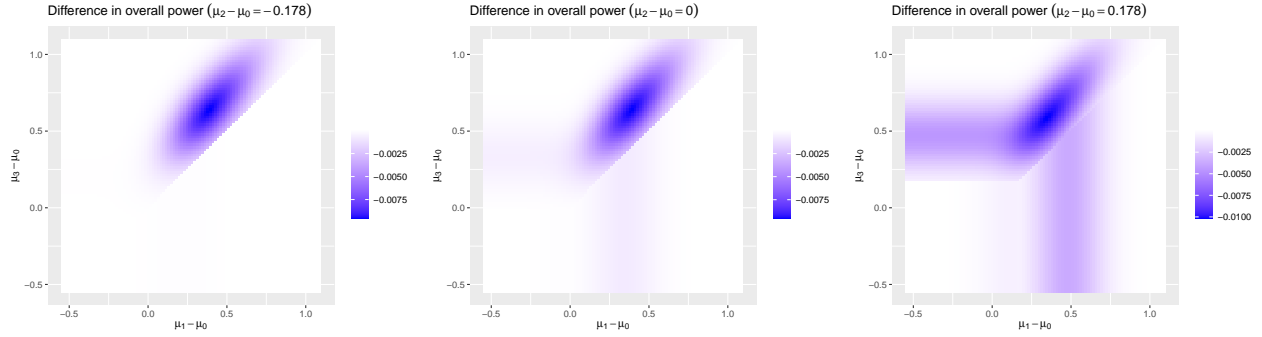

Figure 24: For multiple values of  $\mu_2 - \mu_0$  with treatment 3 added later: the difference in overall power between keeping the data pre change and not.

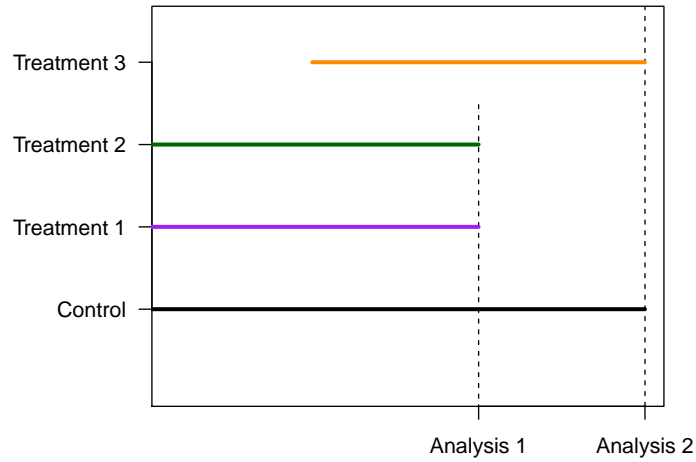

Figure 25: Illustration of the motivating trial when one treatment starts after the first stage and all the treatments only have one analysis.

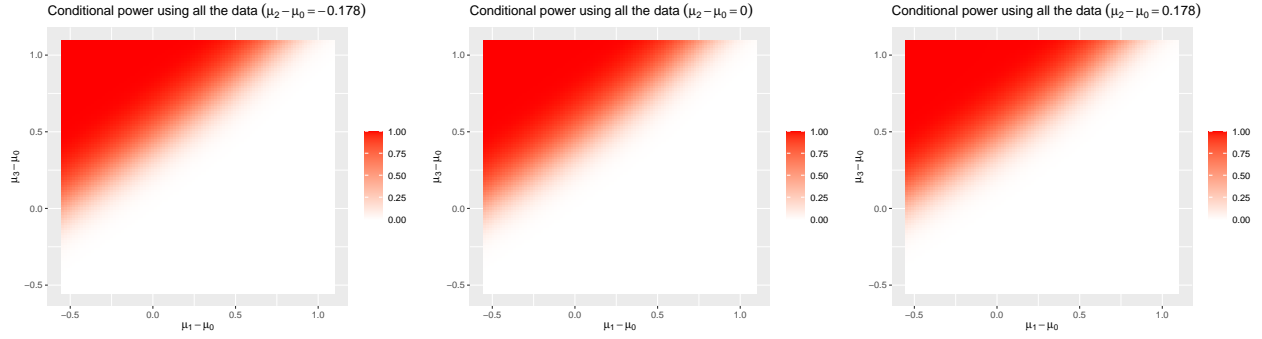

Figure 26: For multiple values of  $\mu_2 - \mu_0$  with treatment 3 added later and each treatment only has 1 analysis: the conditional power for treatment 3 given that treatment 1 has gone forward when all the data is retained.

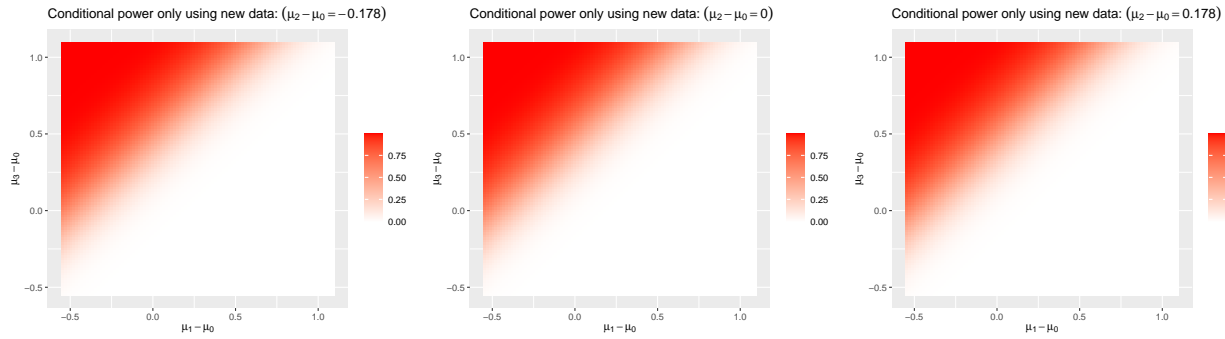

Figure 27: For multiple values of  $\mu_2 - \mu_0$  with treatment 3 added later and each treatment only has 1 analysis: the conditional power for treatment 3 given that treatment 1 has gone forward when only the data post the change in control is used.

in conditional power. As can be seen in Figure 28 now retaining the information can have a positive effect on the conditional power of the trial.

In Figure 29 overall power when comparing treatment 1 and 2 is presented for multiple values of  $\mu_3 - \mu_0$ . The only difference between the overall power when retaining all the data is from treatment 3. Therefore only one set of results when comparing treatment 1 and 2 are presented. However in Figure 30 and Figure 31 the overall power when keeping all the data or only keeping the new data are shown comparing treatment 1 and 3, respectively. In Figure 32 the difference in overall power is shown. This shows in this example there is almost always advantage to keeping the historic data with a power increase of potentially more than 2.5%.

## Competing interests

The authors declare no potential conflict of interests. Alun Bedding is a shareholder of Roche Products Ltd.

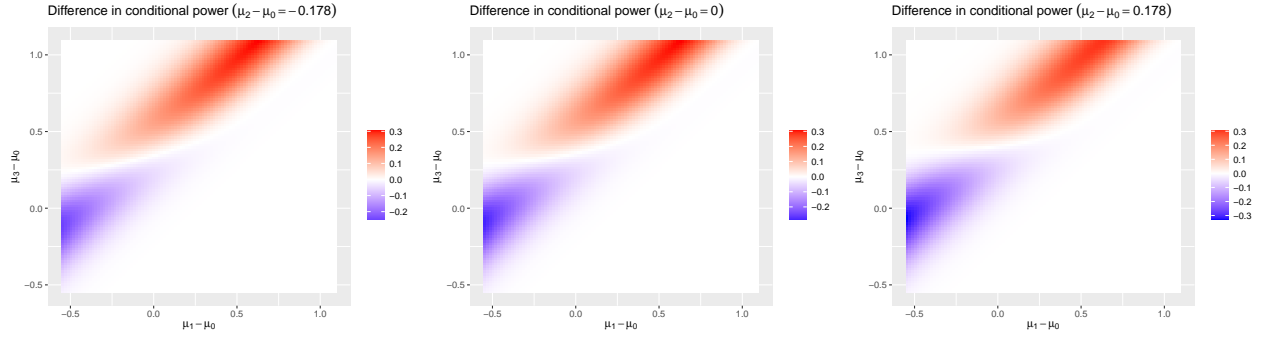

Figure 28: For multiple values of  $\mu_2 - \mu_0$  with treatment 3 added later and each treatment only has 1 analysis: the difference in conditional power between keeping the data pre change and not.

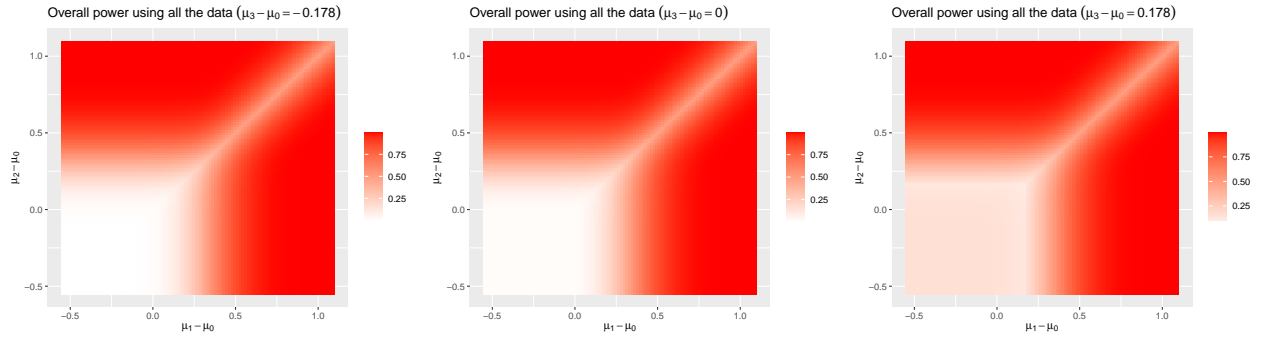

Figure 29: For multiple values of  $\mu_3 - \mu_0$  with treatment 3 added later and each treatment only has 1 analysis: the overall power when only the data post the change in control is used.

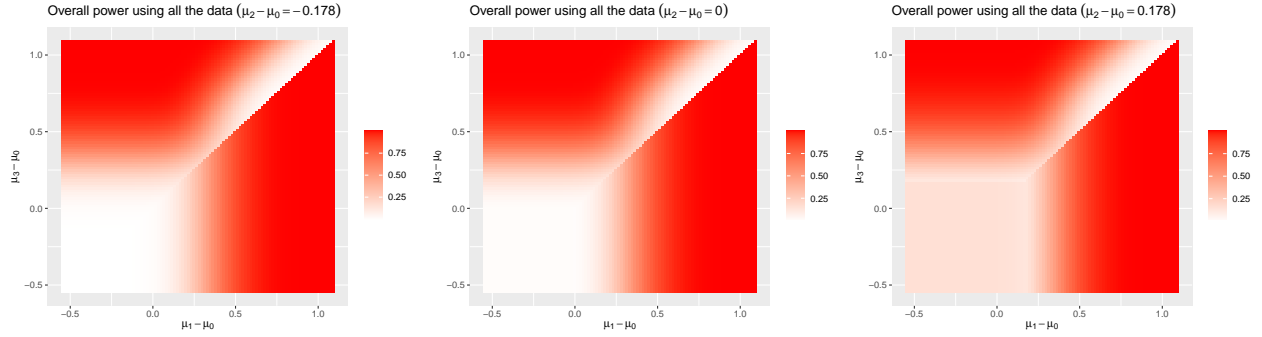

Figure 30: For multiple values of  $\mu_2 - \mu_0$  with treatment 3 added later and each treatment only has 1 analysis: the overall power when all the data is retained.

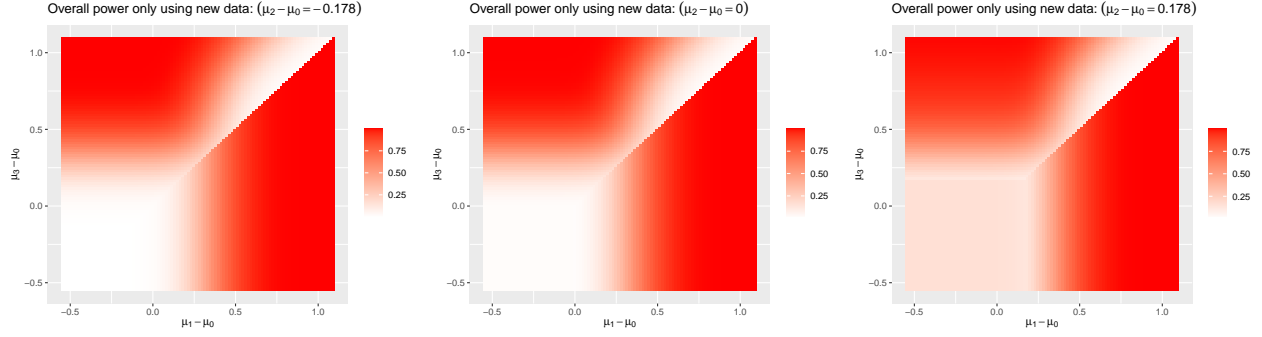

Figure 31: For multiple values of  $\mu_2 - \mu_0$  with treatment 3 added later and each treatment only has 1 analysis: the overall power when only the data post the change in control is used.

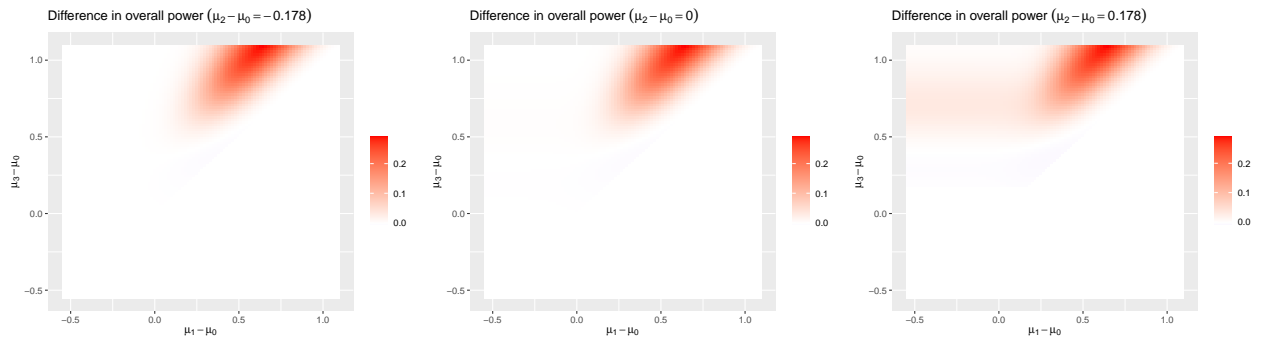

Figure 32: For multiple values of  $\mu_2 - \mu_0$  with treatment 3 added later and each treatment only has 1 analysis: the difference in overall power between keeping the data pre change and not.

## Acknowledgments

This report is independent research supported by the National Institute for Health Research (NIHR300576). The views expressed in this publication are those of the authors and not necessarily those of the NHS, the National Institute for Health Research or the Department of Health and Social Care (DHSC). TJ and PM also received funding from UK Medical Research Council (MC UU 00002/14 and MC UU 00002/19, respectively). This paper is based on work completed while PG was part of the EPSRC funded STOR-i centre for doctoral training (EP/S022252/1). For the purpose of open access, the author has applied a Creative Commons Attribution (CC BY) licence to any Author Accepted Manuscript version arising.

## References

- Greenstreet, P., Jaki, T., Bedding, A., Harbron, C., and Mozgunov, P. (2021). A multi-arm multi-stage platform design that allows pre-planned addition of arms while still controlling the family-wise error. *arXiv preprint arXiv:2112.06195*.
- Greenstreet, P., Jaki, T., Bedding, A., and Mozgunov, P. (2023). A preplanned multi-stage platform trial for discovering multiple superior treatments with control of FWER and power. *arXiv preprint arXiv:2308.12798*.
- Magirr, D., Jaki, T., and Whitehead, J. (2012). A generalized Dunnett test for multi-arm multi-stage clinical studies with treatment selection. *Biometrika*, 99(2):494–501.
- O’Brien, P. C. and Fleming, T. R. (1979). A Multiple Testing Procedure for Clinical Trials. *Biometrics*, 35(3):549–556.
